# Supplementary material for: Spin nematic order in antiferromagnetic spinor condensates
Source: arXiv:1506.06176 source file (2016-04-19)
Supplement: Supplementary file 1 [file SuppInfoResub.pdf]

# Supplementary Material for : Spin nematic order in antiferromagnetic spinor condensates

T. Zibold,<sup>1</sup> V. Corre,<sup>1</sup> C. Frapolli,<sup>1</sup> A. Invernizzi,<sup>1</sup> J. Dalibard,<sup>1</sup> and F. Gerbier<sup>1</sup>

<sup>1</sup>*Laboratoire Kastler Brossel, Collège de France, CNRS, ENS-PSL Research University, UPMC-Sorbonne Universités, 11 place Marcelin Berthelot, 75005 Paris*

(Dated: October 9, 2015)

## I. EXPERIMENTAL SEQUENCE AND PREPARATION

### A. Evaporative cooling of a spin mixture

*a. Preparation of a spin mixture with well-defined magnetization:* Our experimental sequence starts with a pre-cooled thermal cloud of  $^{23}\text{Na}$  atoms in a crossed optical dipole trap [1]. The atomic cloud is partially magnetized, with a magnetization  $m_z \approx 0.5$  resulting from previous cooling steps. We adjust the magnetization by either demagnetizing the atoms further with resonant RF-magnetic field sweeps, or by magnetizing it by evaporation in a magnetic field gradient (“spin distillation”) [2]. We are able to produce final magnetizations ranging from  $\bar{m}_z = 0$  to  $\bar{m}_z = 1$ , with a typical error of 2 – 3 %.

*b. Evaporative cooling in a crossed dipole trap:* After preparing a spin mixture well above the critical temperature for Bose-Einstein condensation, the depth of the optical trap is lowered in a few seconds to perform evaporative cooling. A hold time of 3 s is added after the end of the ramp to ensure that the cloud reaches equilibrium [2]. At the end of the evaporation ramp, the atoms are confined in the crossings of the two beams of the dipole trap, where the trapping potential is well-approximated by a harmonic trap with average trap frequency  $\bar{\omega}/2\pi \sim 405$  Hz (the trap frequencies are in the ratio 1 : 0.85 : 0.5).

Experiments reported in the main article are performed with “almost pure” Bose-Einstein condensates (BECs) containing typically 7500 atoms at a trap depth  $V_T/k_B \approx 400$  nK. By “almost pure”, we mean that no discernible thermal component can be observed in absorption images. Figure S1 shows the measured condensed fraction  $f_c = N_c/N$  for different trap depths  $V_T$  (which sets the temperature obtained by evaporative cooling). The condensed fraction is obtained by fitting a bimodal profile to absorption images of the cloud following the standard procedure [3]. Here  $N$  and  $N_c$  denote respectively the total number of atoms and of condensed atoms, irrespective of their internal state. For condensed fractions larger than  $f_c \approx 0.8$  the contribution of the thermal component becomes difficult to detect, and the bimodal fitting procedure unreliable. This sets a lower bound  $f_c \geq 0.8$  on the condensed fraction for experiments performed without a discernible thermal component.

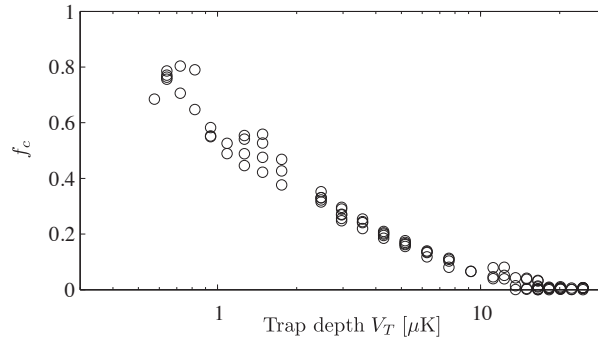

FIG. S1: Condensed fraction versus trap depth, extracted from a fit of a bimodal distribution to the absorption images. The fit function is the sum of a Bose-Einstein thermal distribution for the thermal component and of a Thomas-Fermi profile for the condensate [3].

*c. Stern-Gerlach imaging:* The three Zeeman components are imaged after releasing the cloud from the trap in the presence of a magnetic force separating the Zeeman components. Specifically, we apply a quadrupole field  $\mathbf{B}_q = b'(2x\mathbf{e}_x - y\mathbf{e}_y - z\mathbf{e}_z)$  together with a uniform “separation” field  $B_x\mathbf{e}_x$ , with  $b' \approx 7$  G/cm and  $B_x \approx 3$  G. The resulting adiabatic magnetic potential is given by  $U_{\text{mag}} = g_F m_F \mu_B |B_x \mathbf{e}_x + \mathbf{B}_q| \approx g_F m_F \mu_B |B_x| + g_F m_F \mu_B b' x + \dots$ , with  $g_F = -1/2$  the Landé factor and with  $\mu_B$  the Bohr magneton. The quadrupole and separation field are ramped

up in a few milliseconds, while the bias field  $B_{e_z}$  applied during the experiment is simultaneously ramped down. The timing of the sequence is shown in Figure S3a.

### B. Experimental implementation of Rabi oscillations

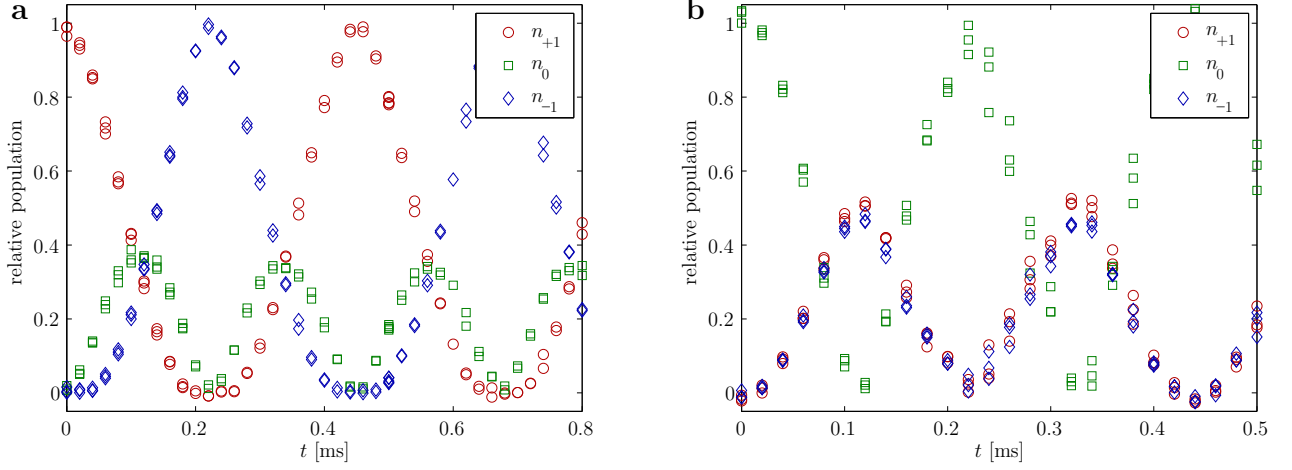

FIG. S2: Rabi oscillation starting either from a state with all atoms in  $m_F = +1$  (a) or  $m_F = 0$  (b). Unlike the data presented in the main text, the fluctuations are dominated by preparation noise, imperfections in the Rabi rotation parameters and the detection noise, all with roughly comparable contributions.

To drive Rabi oscillations between the three Zeeman sublevels, we prepare condensates at a chosen bias magnetic field  $B_z$  in the  $z$  direction and apply a pulse of radio-frequency (rf) magnetic field at the Larmor frequency in the  $y$  direction. The bias field is taken small enough to allow us to neglect the quadratic Zeeman shift ( $q < 100$  Hz) compared to the Rabi frequency ( $\Omega/2\pi \sim 5$  kHz). At the end of the pulse, the separation field  $B_x e_x$  is increased first, followed by the magnetic gradient used for SG imaging and by the decrease of the bias field  $B_z e_z$ . The timing of the sequence is shown in Figure S3a. Ramping up the separation field  $B_x$  is done with a linear ramp of  $T = 3$  ms duration, sufficiently slowly to remain adiabatic with respect to spin flips ( $\omega_L T \ll 1$ ). The optical trap is switched off 10 ms after the end of the RF pulse (see Section IC below).

We have tested this sequence in two special cases, where all the atoms are initially in the  $m_F = +1$  state and or in the  $m_F = 0$  state. We are able to prepare these two states to a very good approximation thanks to the sequence presented before (resulting in  $\Delta m_z \lesssim 1\%$  in these cases). In these two situations there are no fluctuations of the magnetization after rotation due to randomness in the initial state, in contrast to the cases studied in the main paper. The measured oscillations are presented in Figure S2. The contrast is close to 100 %, showing that the assumption of adiabatic following when ramping up the different magnetic fields is valid, and we do not observe any sizable spread of the oscillations after several Rabi periods. This shows that the assumption of adiabatic following when ramping up the different magnetic fields is valid. A key point to achieve good reproducibility of the oscillations has been to synchronize the start of the RF pulse to the 50 Hz oscillations of the mains line frequency.

### C. Influence of spin mixing after the spin rotation

The sudden change of the spin state due to the spin rotation should in principle trigger a spin oscillation dynamics [4–8] driven by spin-exchange interactions during the 10 ms hold time following the spin rotation. As seen before, the applied magnetic field is also changed after the spin rotation, from  $\mathbf{B} = B_z \mathbf{e}_z$  to  $\mathbf{B} = B_z \mathbf{e}_z + B_x \mathbf{e}_x$ . The quadratic Zeeman energy  $q$  increases during this ramp, according to the curve shown in Fig. S3b. This increase is fast compared to the time scale set by spin-exchange interactions,  $\hbar/U_s \sim 25$  ms, and it reduces spin-mixing dynamics due to exchange collisions that would otherwise develop during the 10 ms hold time after the RF pulse. Nevertheless, as seen below, a residual dynamics still takes place and modifies slightly the population  $n_0$  measured in SG imaging. Note that the effect of the spin interaction during the RF pulse is negligible ( $U_s/\hbar\Omega \sim 0.008$ ).

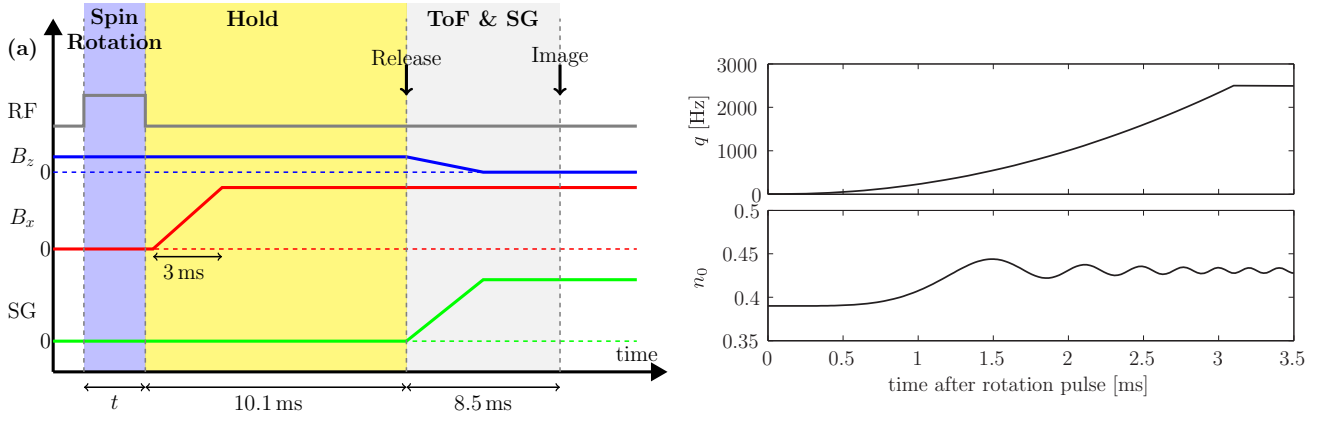

FIG. S3: **(a)**: Schematic diagram (not to scale) showing the experimental sequence. “RF” indicates the rf pulse inducing spin rotations,  $B_z$  is the bias field applied before and during the spin rotation,  $B_x$  and “SG” denote respectively the “separation field” and magnetic field gradient required for SG imaging. **(b)** The ramp of  $B_x$  after the spin rotation results in a time-dependent Quadratic Zeeman energy (QZE)  $q$  increasing within 3 ms after the end of the rf pulse (top panel). The evolution after the spin rotation of the normalized population  $n_0$  due to spin-mixing interactions calculated from Eq. (s2) is shown in the lower panel. The initial relative angle  $\Theta$  was assumed to be  $\pi$ , and the initial population chosen such that the final population is given by  $n_0 \approx 0.43$  as measured in data set *a*. The spin exchange interaction energy was taken to be  $U_s/h = 38$  Hz (see section ID).

To quantify the impact of spin-mixing oscillations on the measured  $n_0$ , we use the theoretical framework given in [7]. The evolution of an initial state

$$|\zeta_i\rangle = \begin{pmatrix} \sqrt{\frac{1-n_{0,i}+m_z}{2}} e^{i(\Theta_i+\alpha)/2} \\ \sqrt{n_0} \\ \sqrt{\frac{1-n_{0,i}-m_z}{2}} e^{i(\Theta_i-\alpha)/2} \end{pmatrix}. \quad (\text{s1})$$

is described by the two Josephson-like equations [7],

$$\hbar \frac{dn_0}{dt} = 2U_s n_0 \sqrt{(1-n_0)^2 - m_z^2} \sin(\Theta), \quad (\text{s2})$$

$$\hbar \frac{d\Theta}{dt} = -2q(t) + 2U_s(1-2n_0) + 2U_s \frac{(1-n_0)(1-2n_0) - m_z^2}{\sqrt{(1-n_0)^2 - m_z^2}} \cos(\Theta), \quad (\text{s3})$$

with  $n_0(0) = n_{0,i}$ , with  $\Theta(0) = \Theta_i$  and with  $q(t)$  as shown in Fig. S3b.

We solve Eqs. (s2) numerically to compute the evolution of  $n_0$ . An example for  $\Theta_i = \pi$  is shown in Fig. S3. The main changes in  $n_0$  occur early in the ramp. Once  $q$  has settled at its final value  $q_f \sim h \times 2.5$  kHz, the dynamics continue as a small amplitude oscillation of the population  $n_0$  around an offset value. These residual oscillations correspond to the quadratic Zeeman regime studied in details in [6]. Their amplitude is small ( $\sim U_s/q_f \sim 0.015$ ) and comparable to our detection noise. Changing the magnetic field to higher values would further reduce the oscillation amplitude, without significantly changing the offset of  $n_0$ . Taking the long-time offset as the measured value of  $n_0$ , we find that the effect of the ramp amounts to *increase* the relative population in  $n_0$  from its initial value by up to 0.05 for an initial angle  $\Theta_i = \pi$ , a small but measurable change.

We emphasize that the spin-mixing dynamics does not change the magnetization  $m_z$  of the system, but only the individual populations  $n_{m_F}$ . Therefore, the occurrence of spin mixing does not influence the analysis of the variance of  $m_z$  after spin rotation. On the other hand, it does affect the maximum likelihood analysis, as detailed further in section IV.

#### D. Determination of $U_s$ from spin-mixing dynamics

We have measured directly the exchange interaction parameter  $U_s$  by deliberately inducing spin-mixing dynamics and recording the oscillations of the normalized population  $n_0$  after a sudden change (see Fig. S4a). Starting from a condensate with all atoms in the  $m_F = 0$  state, prepared as explained above at a bias field  $B \approx 282$  mG [ $q/h \approx 22$  Hz],

we first apply a spin rotation to produce a mixture with roughly balanced populations in all Zeeman states. This results in an initial state as given by Eq. (s1), with  $n_{0,i} \approx 0.38$  and  $m_z \approx 0$ . Spin-changing collisions produce high-contrast oscillations in the Zeeman populations, as observed in previous work for  $m_z \neq 0$  [5, 6, 8, 9]. The oscillation period has been predicted analytically in [7], and is a function of  $n_{0,i}, m_z, q$ , which are known, and of  $U_s$ , which is not. We extract  $U_s/h \approx 38$  Hz from the data by comparing the oscillations period  $T_{\text{osc}} \approx 16$  ms, obtained by a fit to the data to this prediction (see Fig. S4b).

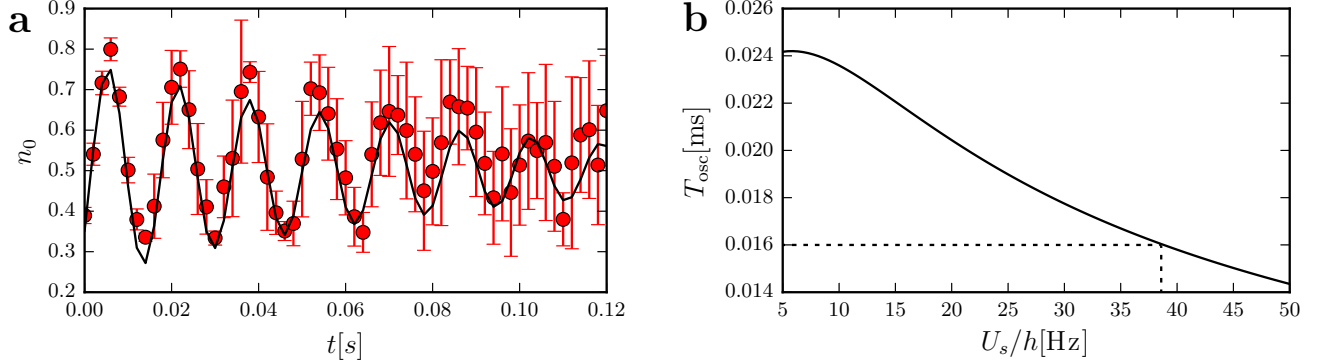

FIG. S4: Spin-mixing oscillations (a) and calculated oscillation period (b). A fit to a damped sinusoid is shown in (a) as solid line, and yields an oscillation period  $T_{\text{osc}} \approx 16$  ms indicated by dashed lines in (b).

### E. Description of the data sets

In total we have taken three data sets for different initial magnetizations and magnetic fields which we label  $a, b, c$  (see Fig. 5 in the main text). The experimental parameters were:  $a$ :  $\bar{m}_z = 0.33$ ,  $q/h = 6.00$  Hz;  $b$ :  $\bar{m}_z = 0.73$ ,  $q/h = 33.7$  Hz;  $c$ :  $\bar{m}_z = 0.71$ ,  $q/h = 3.84$  Hz. We show the results for these data sets in section III C and IV E.

## II. EQUILIBRIUM STATE AT FINITE TEMPERATURES

### A. Finite temperature description of a spinor condensate

In the main text, the initial spin state in equilibrium is described in terms of a zero temperature mean field state  $|\zeta^N\rangle$ , with  $N$  atoms occupying the single-particle spin 1 state

$$|\zeta\rangle = \begin{pmatrix} \sqrt{\frac{1-n_0+m_z}{2}} e^{i(\Theta+\alpha)/2} \\ \sqrt{n_0} \\ \sqrt{\frac{1-n_0-m_z}{2}} e^{i(\Theta-\alpha)/2} \end{pmatrix}. \quad (\text{s4})$$

In a recent paper [10], we have generalized this description to a finite temperature spin ensemble, which was shown to be described to leading order in the small parameter  $1/N$  by the density operator

$$\hat{\rho} \approx \frac{1}{\mathcal{Z}} \int e^{-\beta K} |\zeta^N\rangle \langle \zeta^N| d\zeta, \quad (\text{s5})$$

with  $d\zeta = dn_0 dm_z d\Theta d\alpha$ ,  $\mathcal{Z}$  the partition function and  $\beta = 1/k_B T$  the inverse temperature. The generalized free energy  $K$ , accounting for the conservation of magnetization, can be written as

$$\beta K = \frac{\beta'_z}{2} (m_z - m_z^*)^2 - N\beta q n_0 + N\beta U_s n_0 \left( 1 - n_0 + \sqrt{(1-n_0)^2 - m_z^2} \cos(\Theta) \right). \quad (\text{s6})$$

We have introduced two Lagrange multipliers  $\beta'_z, m_z^*$  determined by the two constraints  $\bar{m}_z = \frac{1}{\mathcal{Z}} \int m_z e^{-\beta K} d\zeta$  and  $\Delta m_z^2 = \frac{1}{\mathcal{Z}} \int (m_z - \bar{m}_z)^2 e^{-\beta K} d\zeta$ .

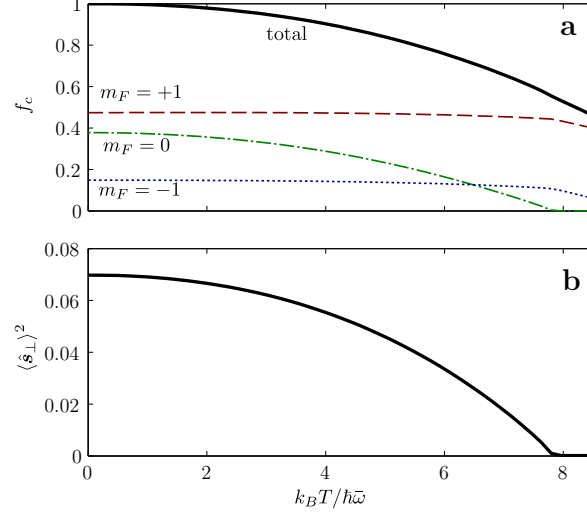

FIG. S5: **(a)** Condensed fraction normalized to the total number of atoms for each Zeeman component  $m_F = +1$  (dashed red),  $m_F = 0$  (dash dotted green) and  $m_F = -1$  (dotted blue line) and total condensed fraction (black solid). **(b)** Total transverse spin length  $\langle \hat{s}_\perp \rangle^2$  versus temperature. The contribution of the thermal cloud is found to be negligible in this scenario. The calculation was done for a spherical trap of frequency  $\omega/(2\pi) = 405$  Hz,  $N = 7500$  atoms,  $\bar{m}_z = 0.33$  and  $q/h = 6$  Hz. In physical units,  $k_B T = 8\hbar\omega$  corresponds to  $T \approx 150$  nK.

Close to the phase transition at  $q_c \approx U_s \left(1 - \sqrt{1 - \bar{m}_z^2}\right)$ , the population  $n_0^* > 0$  which minimizes the free energy is small. An expansion around  $(n_0, m_z) = (n_0^*, \bar{m}_z)$  leads to

$$\beta K \approx \frac{\beta'_z}{2} (m_z - \bar{m}_z)^2 + \beta' \frac{q_c}{U_s \sqrt{1 - \bar{m}_z^2}} (n_0 - n_0^*)^2 + \frac{\beta'}{2} n_0^* \sqrt{1 - \bar{m}_z^2} (\Theta - \pi)^2 + \dots \quad (\text{s7})$$

Equations (s5,s7) show that the initial distribution can be approximated by a Gaussian distribution in  $n_0, m_z, \Theta$ , provided the fluctuations and  $n_0^*$  are small [10].

### B. Hartree-Fock description of the uncondensed component

The single-mode approximation only describes the lowest energy “spatial mode” into which the atoms condense. Higher energy modes can be thermally populated, leading to a *condensed fraction*  $f_c$  lower than one. The thermal component interacts with the condensate and in principle could also develop a magnetic behavior. To describe the thermal component of the non-condensed cloud, we have adapted the Hartree-Fock (HF) description proposed in [11] in the uniform case to our experimental situation.

The model of [11] treats the non-condensed cloud as a gas of non-interacting free particles evolving in a self-consistent mean field potential accounting for spin-exchange interactions [11]. Importantly, this mean field potential is not diagonal in the Zeeman basis due to spin-mixing interactions. The thermal component can in principle develop non-zero coherences due to interactions with the condensate and therefore a non-zero average spin. The quantity of interest is the single-particle density matrix

$$\rho_{m,n}^{(1)}(\mathbf{r}) = \phi_m^*(\mathbf{r})\phi_n(\mathbf{r}) + \rho_{m,n}'^{(1)}(\mathbf{r}), \quad (\text{s8})$$

with  $\phi$  the condensate wavefunction, with  $\rho_{m,n}'^{(1)}$  the contribution of the thermal component, and where  $m, n = 0, \pm 1$ . The density in each Zeeman component  $m$  is determined by the diagonal terms  $\rho_{m,m}^{(1)}$  and the transverse spin by the off-diagonal coherences  $\rho_{0,\pm 1}^{(1)}$ .

With respect to the full HF model laid out in [11], we make two additional simplifying assumptions. First, we assume that the single-mode approximation holds [? ]. This amounts to setting  $\phi_m(\mathbf{r}) = \sqrt{N_c} \bar{\phi}(\mathbf{r}) \zeta_m$ , as done in the

main text. The single mode wavefunction  $\bar{\phi}$  determining the condensate spatial distribution is computed numerically by solving the GP equation

$$\mu\bar{\phi} = -\frac{\hbar^2}{2M_{\text{Na}}}\Delta\bar{\phi} + V(\mathbf{r})\bar{\phi} + \bar{g}N_c|\bar{\phi}|^2\bar{\phi}. \quad (\text{s9})$$

with  $M_{\text{Na}}$  the mass of Sodium atoms. The spinor part  $\zeta_m$  is found from the single-mode theory using  $U_s = N_c g_s \int d^{(3)}\mathbf{r} |\bar{\phi}|^4$ . The coupling constants  $\bar{g}, g_s$  are proportional to the scattering lengths  $\bar{a} \approx 2.79 \text{ nm}$  and  $a_s \approx 0.1 \text{ nm}$  [12] with a proportionality factor  $4\pi\hbar^2/M_{\text{Na}}$ . Second, we neglect the interaction energy of the thermal cloud in comparison to the one of the condensate (“semi-ideal” model [13]). Far from  $T_c$ , this is expected to be an accurate approximation [14]. Finally, we perform the calculations for a spherical trap. Although the trapping potential used in the experiment is not exactly isotropic, we do not expect that this affects strongly the results (in the Thomas-Fermi regime, for instance, only the average trap frequency matters to compute thermodynamic quantities [14]).

The excitations modes  $\mathbf{u}^{(\nu)}$  and energies  $E_\nu$  are solutions of the eigenproblem

$$E_\nu \mathbf{u}^{(\nu)} = \left( -\frac{\hbar^2}{2M_{\text{Na}}} \Delta \cdot + V(\mathbf{r}) + A(\mathbf{r}) \right) \mathbf{u}^{(\nu)} \quad (\text{s10})$$

where the matrix  $A$ , explicitly given in [11], depends on the condensate wavefunction  $\phi(\mathbf{r})$  and on  $\bar{g}, g_s$ . Diagonalizing this equation, we obtain the single-particle density matrix  $\rho^{(1)}$  of the thermal component as

$$\rho'_{m,n}(1)(\mathbf{r}) = \sum_{\nu} \left( \mathbf{u}_m^{(\nu)}(\mathbf{r}) \right)^* \mathbf{u}_n^{(\nu)}(\mathbf{r}) N_{\text{BE}}(E_\nu) \quad (\text{s11})$$

with  $N_{\text{BE}}(E) = 1/(e^{E/k_B T} - 1)$  the occupation number for each mode  $\nu$ .

The results of this calculation are shown in figure S5. The parameters were chosen to correspond to the experimental situation of data set *a* in the main article. The condensed fraction in  $m_F = 0$  decreases first. Above  $k_B T \geq 7.8\hbar\omega$ , the  $m_F = 0$  component is purely normal and the condensate is formed by  $m_F = \pm 1$  only. The transverse spin is reduced with increasing temperature. As found in [11], the contribution of the thermal component to the average spin vector is oriented opposite to the average spin of the condensate. The transverse spin is thus naturally reduced with increasing temperature. In the regime we have investigated, the temperatures fulfill  $k_B T \gg q, U_s$ . As a result, the non-condensate spin vector is always much smaller in magnitude than its condensed counterpart, and we find that the main effect that reduces the length of the transverse spin vector is the reduction of the condensed fraction. For a total condensed fraction  $f_c = 0.8$  the transverse component  $\langle \hat{s}_\perp \rangle^2$  of the spin is reduced to about 57% of its zero temperature value, corresponding to the lower limit of the shaded area in figure 3 of the main text. The data are closer to a value  $f_c \approx 0.9$ .

### III. SPIN ROTATIONS AND SPIN NOISE

#### A. Theoretical description of spin rotations

We compute the effect of the spin rotation using the standard angular momentum algebra. In a Rabi-type experiment where a resonant RF field polarized along  $y$  is applied at  $t = 0$  and in the rotating-wave approximation, the evolution operator is equivalent to a rotation operator along  $y$  with a rotation angle  $\Omega t$  proportional to the pulse length  $t$  and to the Rabi frequency  $\Omega$ . The state  $\Psi$  of a single spin 1 atom transforms under rotation as

$$|\Psi'\rangle = e^{-i\Omega t \hat{S}_y} |\Psi\rangle = \hat{R}_y(\Omega t) |\Psi\rangle. \quad (\text{s12})$$

Here and in the following, primed variables denote quantities evaluated after the spin rotation is complete. The relevant rotation matrix for a spin 1 is given by

$$\hat{R}_y(\Omega t) = \mathbb{1} - i \sin(\Omega t) \hat{S}_y + (\cos(\Omega t) - 1) \hat{S}_y^2 \quad (\text{s13})$$

The populations of each Zeeman state after the pulse are given by simple expressions when starting from  $|m_F = +1\rangle$ ,  $|\Psi'_{+1}|^2 = \cos^4(\frac{\Omega t}{2})$ ,  $|\Psi'_{-1}|^2 = \sin^4(\frac{\Omega t}{2})$ , and  $|\Psi'_0|^2 = \sin^2(\Omega t)/2$ . Similarly, for an initial state  $|m_F = 0\rangle$ , one has  $|\Psi'_{+1}|^2 = |\Psi'_{-1}|^2 = \frac{1}{2} \sin^2(\Omega t)$  and  $|\Psi'_0|^2 = \cos^2(\Omega t)$ .

### B. General formula for the spin variance

We derive in this section a general formula linking the moments of the magnetization *after rotation* to properties of the initial states. We apply the rotation to the spin operator  $\hat{S}_z$ , and make use of the angular momentum algebra to obtain,

$$\hat{S}'_z = \hat{R}_y^\dagger(\Omega t) \hat{S}_z \hat{R}_y(\Omega t) = \cos(\Omega t) \hat{S}_z - \sin(\Omega t) \hat{S}_x. \quad (\text{s14})$$

We now introduce a key assumption: the initial density matrix is invariant under rotation around the  $z$  axis, or, using the notations in the main article, the phase  $\alpha$  is random from one realization of the experiment to the next (with a uniform distribution in  $[0, 4\pi]$ ). The value of an observable measured after averaging over many realizations of the experiment is

$$\langle \hat{O} \rangle_\alpha = \frac{1}{4\pi} \int_0^{4\pi} d\alpha \langle \mathcal{R}^\dagger \hat{O} \mathcal{R} \rangle, \quad (\text{s15})$$

where  $\mathcal{R} = e^{-i\Omega t \hat{S}_y} e^{-i\frac{\alpha}{2} \hat{S}_z}$ . The  $\langle \cdot \rangle_\alpha$  symbol is intended to stand for a double average : the first one, denoted by  $\langle \cdot \rangle$ , is the usual average over the quantum state before rotation for each realization, and the second one is done over random values of  $\alpha$  arising from one experimental realization to the next. Defining an average in this way allows us to obtain formula expressing measurement results without specifying the initial state. We have for instance

$$\hat{S}'_z = \mathcal{R}^\dagger \hat{S}_z \mathcal{R} = \cos(\Omega t) \hat{S}_z - \sin(\Omega t) \left( \cos(\alpha/2) \hat{S}_x + \sin(\alpha/2) \hat{S}_y \right). \quad (\text{s16})$$

Using this result, we find the average and variance of  $\hat{S}'_z/N$  after the pulse,

$$\langle m'_z \rangle_\alpha = \frac{1}{N} \langle \hat{S}'_z \rangle_\alpha = \cos(\Omega t) m_z, \quad (\text{s17})$$

$$\Delta m_z'^2 = \cos^2(\Omega t) \Delta m_z^2 + \frac{1}{2N^2} \sin^2(\Omega t) \langle \hat{S}_x^2 + \hat{S}_y^2 \rangle. \quad (\text{s18})$$

In other words, relying only on the randomness of  $\alpha$  we find that the variance of the magnetization  $\Delta m_z'^2$  after the pulse measures the initial transverse spin fluctuations. This result holds for any initial state, and only relies on the fact that the pulse is short enough to neglect any other terms than the oscillating field in the Hamiltonian during the evolution time.

Introducing the squared length  $\langle \hat{\mathbf{s}}_\perp \rangle^2 = (\langle \hat{S}_x \rangle^2 + \langle \hat{S}_y \rangle^2)/N^2$  of the mean transverse spin and  $\Delta s_\perp^2 = \langle \hat{S}_x^2 + \hat{S}_y^2 \rangle/N^2 - \langle \hat{\mathbf{s}}_\perp \rangle^2$  its variance, we obtain our final result

$$\Delta m_z'^2 = \frac{1}{2} \sin^2(\Omega t) \langle \hat{\mathbf{s}}_\perp \rangle^2 + \cos^2(\Omega t) \Delta m_z^2 + \frac{1}{2} \sin^2(\Omega t) \Delta s_\perp^2. \quad (\text{s19})$$

We thus expect that the variance  $\Delta m_z'^2$  oscillates with the rotation angle  $\Omega t$  and reaches its maximum for  $\Omega t = \pi/2$  where the slope of  $m'_z$  versus  $\Omega t$  is maximum. The last two noise terms in Eq. (s19) are typically dominated by the preparation noise on  $m_z$  (which also introduces noise on  $n_0$  in the equilibrium state, and thus on  $\langle \hat{\mathbf{s}}_\perp \rangle$ ).

We note that this measurement gives access to a quantity (the squared transverse spin length) which can be used to characterize other phases than a fully condensed state. The expression

$$\hat{S}_x^2 + \hat{S}_y^2 = N + \hat{N}_0 + 2\hat{N}_0 \left( \hat{N}_{+1} + \hat{N}_{-1} \right) + \left( \hat{a}_{+1}^\dagger \hat{a}_{+1}^\dagger \hat{a}_0^2 + \text{h.c.} \right), \quad (\text{s20})$$

shows that measuring the spin variance gives access to the “spin singlet amplitude”  $\langle \hat{a}_{+1}^\dagger \hat{a}_{+1}^\dagger \hat{a}_0^2 \rangle$  [15, 16], which appears in studies of fluctuating systems beyond mean field (spin liquid in one dimension [17], or spin-singlet Mott states in optical lattices, for instance [18]). The results are also easily generalized beyond the single-mode approximation.

### C. Complementary data sets for the spin variance

We show here additional data sets not shown in the main article, which have been obtained for the parameters located at the points  $b, c$  in the mean field phase diagram (see figure 5 in the main text). Point  $a$  shown in the main



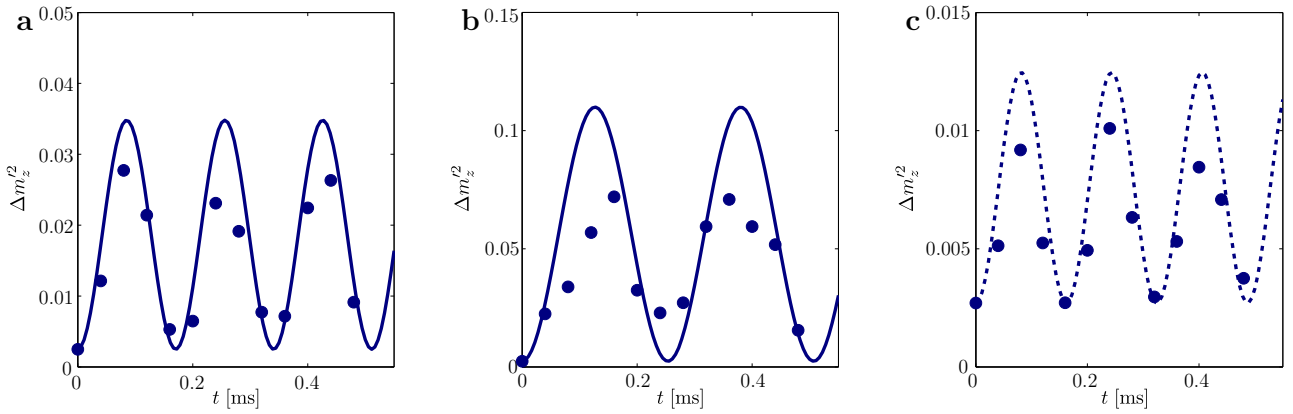

FIG. S6: Variance data for measurements *a*, *b* and *c* (see figure 5 in the main text). In panel (a) and (b) the solid blue line is the zero temperature theory for an initial angle of  $\Theta = \pi$  (antiferromagnetic interactions). Panel (c) shows data set *c* which is below the phase transition line. The zero temperature theory predicts no oscillation in the variance at all since  $n_0$  and thereby  $\langle \hat{s}_\perp \rangle^2$  vanish. The dotted curve is the theoretical expectation from Eq. s19 taking the initial measured  $n_0$  into account (corrected for the effect of the spin-mixing collisions described in Section IC).

article is also reproduced for comparison. The same behavior is observed in all cases, an oscillation of the variance with fixed amplitude.

The case shown in Fig. S6c (data set *c*), taken below the  $T = 0$  phase transition, deserves a separate discussion. According to the  $T = 0$  mean field picture, one would expect  $\bar{n}_0 = 0$  and  $\langle \hat{s}_\perp \rangle^2 = 0$  (see Eq. (2) in the main text). In contrast, we find a small initial population  $n_0 \approx 0.04$ , and an oscillation of the magnetization variance with a small, but non-zero amplitude. The dotted lines in the figure correspond to the theoretical predictions which take the initial measured  $n_0$  into account (corrected for the small shift in  $n_0$  due to the spin changing collisions discussed in Section IC) and  $\Theta = \pi$ .

A first explanation for this behavior could be the presence of the thermal (uncondensed) component. In the Bogoliubov framework [19], spin excitations are phase-locked to the condensed components, and a finite transverse spin originating from the uncondensed component could contribute to our signal. However, from the Hartree-Fock calculations described in Section IIB, we found that the transverse spin of the uncondensed component remains very small for our typical parameters, and cannot explain the measured signal.

A second explanation comes from a finite temperature of the initial spin state of the condensate, which is then described by a statistical ensemble rather than a pure state [10]. This leads to a finite population in  $m_F = 0$  even below the phase transitions [10]. By numerically integrating the thermal distribution described by the free energy in Eq. (s6) for a typical temperature  $k_B T = 80$  nK, we find a finite population  $\bar{n}_0 = 0.016$ . This leads to a maximal variance after rotation of  $\Delta m_z^2 = 0.005$ . Although this is smaller than the observed fluctuations we want to emphasize that the amplitude of the variance oscillations found still indicates to the antiferromagnetic order of the state with  $\Theta = \pi$ . Our maximum likelihood estimation algorithm also agrees with these findings as is shown in the next section.

## IV. MAXIMUM LIKELIHOOD ESTIMATION OF THE DISTRIBUTION OF $\Theta$

### A. Principle of the method

The maximum likelihood estimation (MLE) provides an estimator for an unknown parameter by comparing the outcome of a measurement with a model distribution depending on the unknown parameter. The comparison attributes a likeliness to each parameter value, by evaluating the model distribution at the result of the measurement. The best estimated parameter given the set of measurements corresponds to the value which maximizes the likelihood function. Since the estimator strongly depends on the chosen probabilistic model, it is important for the model to be close to the physical reality. In the following we motivate the model chosen for our measurement.

In our case the measurement data consists of couples  $(m'_{z,i}, n'_{0,i})$  which we find after various rotation angles  $\{\Omega t_i\}$  corresponding to evolution times  $\{t_i\}$  in the RF field. In the framework of MLE, the measurement results are seen as probabilistic variables of an unknown probability distribution. We model this distribution by a set of probability distributions which we derive from the knowledge about our initial state, its transformation during the Rabi rotation



and independently measured experimental noise.

### B. Model for the initial distribution

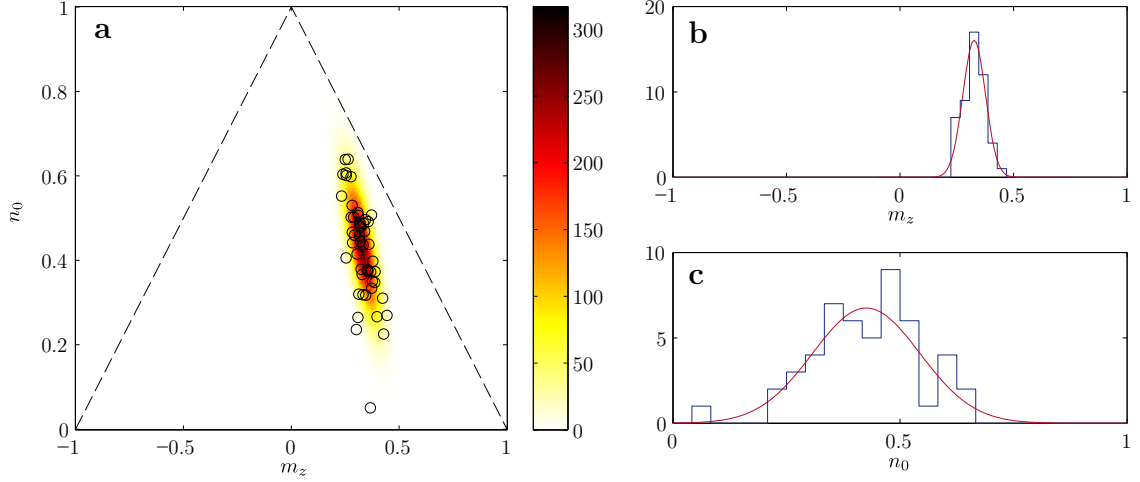

FIG. S7: Initial distribution of the populations  $n_0$  and  $m_z$  for data set *a*. **(a)** Measured initial populations are indicated by black circles. Color-coded is the 2D-histogram of the simulated  $10^6$  initial points used in the Monte Carlo method with linear bin width  $2.5 \times 10^{-3}$ . The initial 2D-Gaussian distribution is estimated from the initial measurements. The dashed lines limit the allowed area ( $|m_z| \leq 1 - n_0$ ). Marginal histograms of measured initial populations for  $m_z$  **(b)** and  $n_0$  **(c)**. The red line indicates the marginal distributions used for the Monte Carlo analysis.

The distribution of initial states is probabilistic due to three different effects. The first effect is intrinsic to our theoretical model which is degenerate in the initial angle  $\alpha$ . We therefore expect that it takes random values from realization to realization with a uniform distribution.

The second probabilistic effect is due to experimental imperfections. In an ideal scenario the parameters  $n_0$  and  $m_z$  characterizing the initial state  $\zeta$  would be fully determined by minimizing the mean field energy. In our experiment however we find fluctuations of these parameters from realization to realization. The fluctuations of  $m_z$  result from experimental imperfections in our preparation process and in the subsequent evaporation. Assuming the cloud reaches equilibrium before we probe it with spin rotation, fluctuations in  $m_z$  or in the spin-spin interaction energy  $U_s$  (due to fluctuations of the total atom number or of the confinement strength) result in correlated fluctuations in  $n_0$  due to the system exploring different minima of the mean field energy.

A third probabilistic mechanism originates from the finite spin temperature as described in Section II A which allows the system to explore states situated away from the minimum. The second and third effect are more pronounced close to the phase transition [10]. In principle, one could account for both by convolving the initial finite temperature density matrix  $\hat{\rho}$  by the probability distribution describing preparation noise on  $m_z$  and the correlated fluctuations of  $n_0$ . For our setup, we estimate that experimental imperfections dominate (in the language of Section II A,  $\beta'_z \ll \beta'$ ) and we include only the latter effect.

We find empirically that the initial joint distribution of  $n_0$  and  $m_z$  is well described by a two-dimensional Gaussian  $\mathcal{G}(n_0, m_z)$ . We thus assume that the initial density operator is of the form

$$\hat{\rho} = \int dn_{0,i} dm_z d\Theta d\alpha \frac{\mathcal{G}(n_{0,i}, m_z) P(\Theta)}{4\pi} |\zeta^N\rangle \langle \zeta^N|. \quad (\text{s21})$$

We stress that  $\mathcal{G}(n_{0,i}, m_z)$  reflects the fluctuations of the preparation, but that the marginal distribution  $P(\Theta)$  is *a priori* not affected by them. At  $T = 0$ ,  $P(\Theta)$  is given by a Dirac delta,  $P(\Theta) \propto \delta(\Theta - \pi)$ , but acquires a finite width at finite  $T$  (see Section IV D below). The mean and covariance matrix characterizing  $\mathcal{G}$  are calculated from the measured data without spin rotation. We account for the spin changing collisions discussed in Section I C, which affect the measured “initial distribution”. Specifically, for each values of  $\Theta$ ,  $m_z$  and  $n_0$ , the mean field equations (s2) are used to find the initial value  $n_{0,i}$  that leads to the measured one,  $n_0$ . The known values of  $q$  and the measured value of  $U_s$  are used as fixed inputs for this calculation. The initial distribution  $\mathcal{G}(n_{0,i}, m_z)$  deduced in this way is shown in Figure S7.

### C. Monte Carlo approach

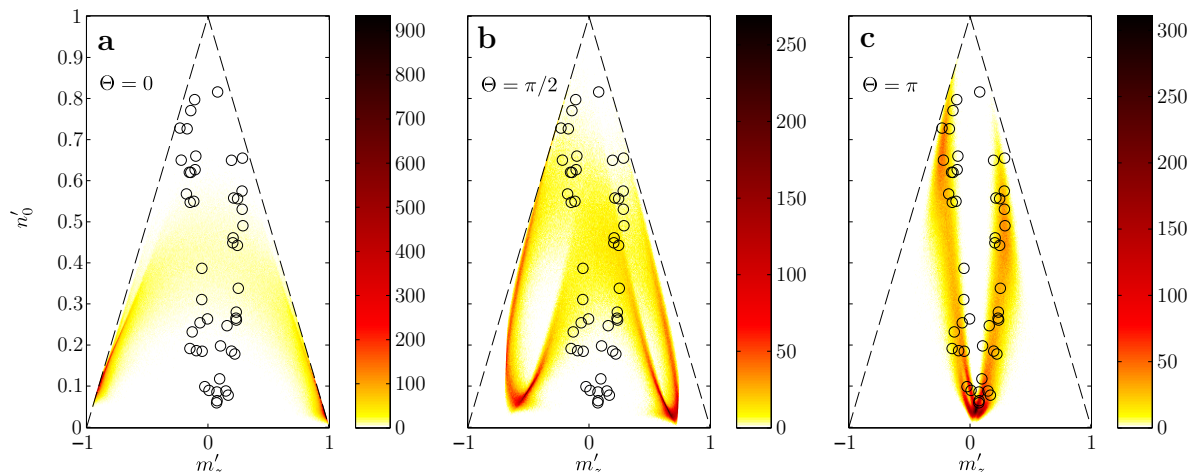

FIG. S8: Comparison for data set *a* of the Monte Carlo simulated populations with measured data (black circles) after Rabi-rotation for different assumed initial angles  $\Theta$ . The three panels show the color-coded 2-D histograms of the Monte Carlo simulations for  $\Theta = 0$  (a),  $\pi/2$  (b) and  $\pi$  (c). Black circles indicate the same measured populations in all panels. Best agreement, *i.e.* the maximum likelihood is found for  $\Theta = \pi$ . The example is taken for  $\Omega t \approx \pi/2$  where sensitivity is the highest.

In order to construct a MLE for the parameters characterizing the distribution  $P(\Theta)$ , we need to obtain a distribution of the measurement outcomes from the knowledge of the initial state, including the evolution under spin rotation and measurement noise on the final Zeeman state populations. We use a Monte Carlo approach, where the initial density operator is sampled by drawing random numbers  $(n_0, m_z, \alpha)$  according to our assumed probability distributions (see figure S7) and assuming a certain value for  $\Theta$ . This determines an initial mean field state  $|\zeta^N\rangle$ . Using the known evolution under spin rotations, we propagate this state in time for a given  $t_i$  to arrive at the final mean outcome populations  $(n'_0, m'_z)$  as the expectation values of the corresponding operators in the time-evolved mean field state. In our numerical implementation we use a typical number of  $\sim 10^6$  Monte Carlo samples to reconstruct the final statistical distribution of the measurement outcomes.

As discussed in Section IC, the spin populations change slightly due to spin-mixing collisions in the beginning of the magnetic field ramp applied just after the spin rotation. This was already included in the determination of the initial distribution of  $(m_z, n_0)$  and we also take this effect into account when comparing with the final simulated distributions. In the Monte-Carlo simulation, the spin state found after rotation is used as initial condition to solve the mean field equations (s2) describing the spin dynamics. We arrive in this way at a distribution of  $n'_0$  corrected for the effect of spin changing collisions. For initial angles close to  $\Theta = \pi$ , the population  $n_0$  changes by a few percents.

By evaluating the final populations using their expectation values, we neglect the quantum fluctuations on the final results, which are on the order  $1/\sqrt{N_{m_F}}$  and small for our typical atom numbers of particles ( $N_{m_F} \sim$  a few thousands) when compared to the noise level of our population measurements. The measurement noise results from a combination of photon shot noise and small spatial intensity fluctuations of the laser pulse used for absorption imaging, and is typically  $\Delta n_{m_F} \approx 1\%$  for the normalized population in Zeeman state  $m_F$ . We include this noise in our model by convolving the simulated measurement outcome by a Gaussian distribution. This leads to a continuous probability density  $p_{t_i}(n'_0, m'_z|\Theta)$  for the measurement outcome which depends on the initial phase  $\Theta$ , and defines the log-likelihood function as described in the main text.

As a side remark, we note that including the spin changing collisions into the MLE analysis changes the symmetry of the final distribution. Without including them, the final distributions  $p_{t_i}(n'_0, m'_z|\Theta)$ , and therefore the likelihood, enjoy a reflection symmetry around  $\Theta = \pi$  and  $\Theta = 0$ . When spin-mixing collisions are taken into account, this symmetry is lost. For comparison, we show in figure S10 not only the likelihoods accounting for the effect of the spin changing collisions (panel a-c) but also the ones which do not include the correction (panel d-f).

### D. Probabilistic model for $\Theta$

We model the marginal distribution  $P(\Theta)$  that is to be estimated by the MLE procedure by a truncated Gaussian with a mean value  $\bar{\Theta}$  and a standard deviation  $\sigma_{\Theta}$ . The finite width can be attributed to two effects. The first effect originates from the finite temperature of the initial spin ensemble, as discussed in Section II A. Eq. (s6) shows that the marginal distribution of  $\Theta$  obtained after integrating over  $n_0, m_z$  is approximately Gaussian, with a root-mean-square (rms) width  $\approx \sqrt{k_B T / N U_s}$ . A numerical integration of the full distribution without approximations for a realistic temperature  $T/k_B \approx 80$  nK and the experimental parameters of data set *a* leads to the distribution shown in Fig. S9, with a width  $\approx 0.1$  comparable to the results of the MLE. The second effect originates from an underestimation of the noise sources in the system. As seen before, the probability distribution  $p_{t_i}(n'_0, m'_z | \Theta)$  is almost symmetric in  $\Theta$  with respect to 0 and  $\pi$ . The presence of fluctuations (induced for example by experimental imperfections) not included in our model always bias the estimator away from  $\Theta = \pi$ . We thus conclude that the finite width of  $P(\Theta)$  probably partly accounts for underestimated or unconsidered noise in our probabilistic model. This conclusion still holds qualitatively when spin-mixing collisions are taken into account and the symmetry of  $L(\Theta)$  around  $\pi$  is lost.

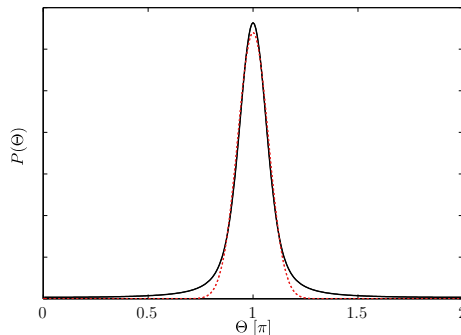

FIG. S9: The black solid line shows the marginal probability distribution for the phase  $\Theta$  for a thermal spin ensemble at a temperature of 80 nK. The distribution was obtained by numerical integration of the thermal distribution described by Eqs. (s5) and (s6) for the parameters of data set *a*. The red dotted line shows the best Gaussian fit.

### E. Additional data analysis with the MLE algorithm

We show here the results found by the MLE approach for the three data sets *a*, *b* and *c* in Fig. S10.

## V. GEOMETRIC CHARACTERIZATION OF SPIN 1 CONDENSATES

### A. Representation of a spin 1 state in the cartesian basis

A given spin 1 state  $|\Psi\rangle$  can be defined in terms of its components  $\{\Psi_{+1}, \Psi_0, \Psi_{-1}\}$  in the standard basis formed by the eigenvectors of  $\hat{s}_z$  with eigenvalues  $+1, 0, -1$ , respectively. For our purpose, it is convenient to use instead the so-called Cartesian basis  $\{|x\rangle, |y\rangle, |z\rangle\}$  defined as  $|x\rangle = \frac{1}{\sqrt{2}}(|-1\rangle - |+1\rangle)$ ,  $|y\rangle = \frac{i}{\sqrt{2}}(|-1\rangle + |+1\rangle)$ , and  $|z\rangle = |0\rangle$ . From the relation  $\hat{S}_a|b\rangle = i\epsilon_{abc}|c\rangle$  ( $\epsilon_{abc}$  is the fully antisymmetric tensor), we deduce that the cartesian state  $|a\rangle$  is the eigenstate of  $\hat{S}_a$  with eigenvalue 0. The spin 1 state in the Cartesian basis can be written as [20–23]

$$|\Psi\rangle = \begin{pmatrix} \frac{1}{\sqrt{2}}(\Psi_{-1} - \Psi_{+1}) \\ \frac{-i}{\sqrt{2}}(\Psi_{+1} + \Psi_{-1}) \\ \Psi_0 \end{pmatrix}_c = (\mathbf{u} + i\mathbf{v}) \cdot |\mathbf{r}\rangle, \quad (\text{s22})$$

where we introduced two real vectors  $\mathbf{u}$ ,  $\mathbf{v}$  that are useful to simplify the algebra. From the normalization  $\mathbf{u}^2 + \mathbf{v}^2 = 1$  alone, the vectors  $\mathbf{u}$  and  $\mathbf{v}$  are not uniquely defined. Performing a gauge transformation  $\Psi \rightarrow \Psi' = e^{i\gamma}\Psi$  transforms  $\mathbf{u}$  and  $\mathbf{v}$  as  $\mathbf{u}' = \cos(\gamma)\mathbf{u} - \sin(\gamma)\mathbf{v}$  and  $\mathbf{v}' = \cos(\gamma)\mathbf{v} + \sin(\gamma)\mathbf{u}$ . As a result, we can choose  $\gamma$  such that  $\mathbf{u} \cdot \mathbf{v} = 0$  and  $|\mathbf{u}| \geq |\mathbf{v}|$ . We make this choice in the following.

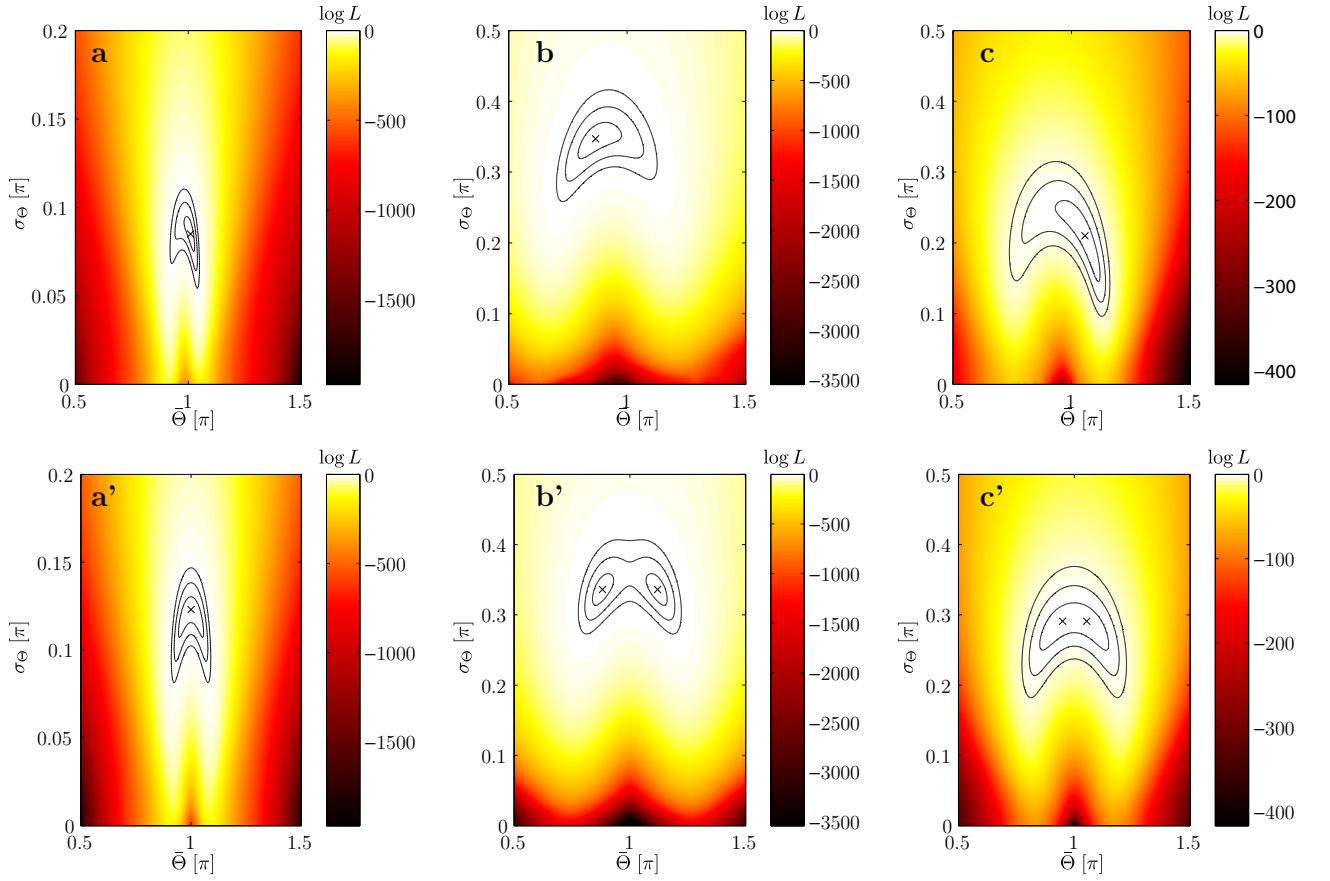

FIG. S10: The first row of panels (a-c) shows the results for the maximum likelihood estimation for the datasets *a*, *b* and *c* (see figure 5 in the main text). In all cases the maximum, *i.e.* the estimated phase  $\Theta$ , is found close to the theoretical predicted value of  $\pi$  (black cross). The contour lines indicate the 67%, 95% and 99% confidence area. The second row of panels (a'-c') shows the corresponding results obtained if the small changes of the  $n_0$  population induced by the residual spin-mixing dynamics (Sec. IC) is ignored. These results quantitatively close to the ones in a-c but are fully symmetric with respect to  $\Theta = \pi$ .

In terms of the unit vectors  $\mathbf{u}$ ,  $\mathbf{v}$ , the average spin vector is  $\langle \hat{\mathbf{s}} \rangle = 2\mathbf{u} \times \mathbf{v}$  and the spin quadrupole tensor  $Q_{ij} \equiv \frac{1}{2} \langle \hat{s}_i \hat{s}_j + \hat{s}_j \hat{s}_i \rangle$  is

$$Q_{ij} = \delta_{ij} - (u_i u_j + v_i v_j). \quad (\text{s23})$$

We introduce three unit vectors  $\{\mathbf{u}, \mathbf{v}, \mathbf{w}\}$  defined as  $\mathbf{u} = \frac{\mathbf{u}}{|\mathbf{u}|}$ ,  $\mathbf{v} = \frac{\mathbf{v}}{|\mathbf{v}|}$ ,  $\mathbf{w} = \frac{\langle \hat{\mathbf{s}} \rangle}{|\langle \hat{\mathbf{s}} \rangle|}$ . Since  $\mathbf{u} \cdot \mathbf{v} = 0$  and  $\mathbf{w} = \mathbf{u} \times \mathbf{v}$ ,  $\{\mathbf{u}, \mathbf{v}, \mathbf{w}\}$  forms an orthonormal, right-handed triad and  $Q_{ij}$  is already diagonal. We can rewrite the spin quadrupolar tensor  $\overline{\overline{Q}}$  in a more geometric form,

$$\overline{\overline{Q}} = \frac{1 - \mathcal{A}}{2} \mathbf{u} \otimes \mathbf{u} + \frac{1 + \mathcal{A}}{2} \mathbf{v} \otimes \mathbf{v} + \mathbf{w} \otimes \mathbf{w}, \quad (\text{s24})$$

where

$$\mathcal{A} = 2|\mathbf{u}|^2 - 1. \quad (\text{s25})$$

A generic spin 1 state is uniquely determined by the average spin vector  $\langle \hat{\mathbf{s}} \rangle$  and by the spin quadrupole tensor  $Q_{ij}$  given above. There are two limiting cases. The first one is the case of an aligned state (also called spin nematic or polar state in the context of spinor condensates [24]), where the spin wavefunction takes the form

$$|\Psi\rangle = \mathbf{u} \cdot |\mathbf{r}\rangle, \quad (\text{s26})$$

*i.e.* is the eigenstate of  $\hat{\mathbf{s}} \cdot \mathbf{u}$  with zero eigenvalue. In such a state, the average spin vanishes,  $|\langle \hat{\mathbf{s}} \rangle| = 0$ , and the spin quadrupole tensor is

$$\overline{\overline{Q}} = \mathbb{1} - \mathbf{u} \otimes \mathbf{u}. \quad (\text{s27})$$

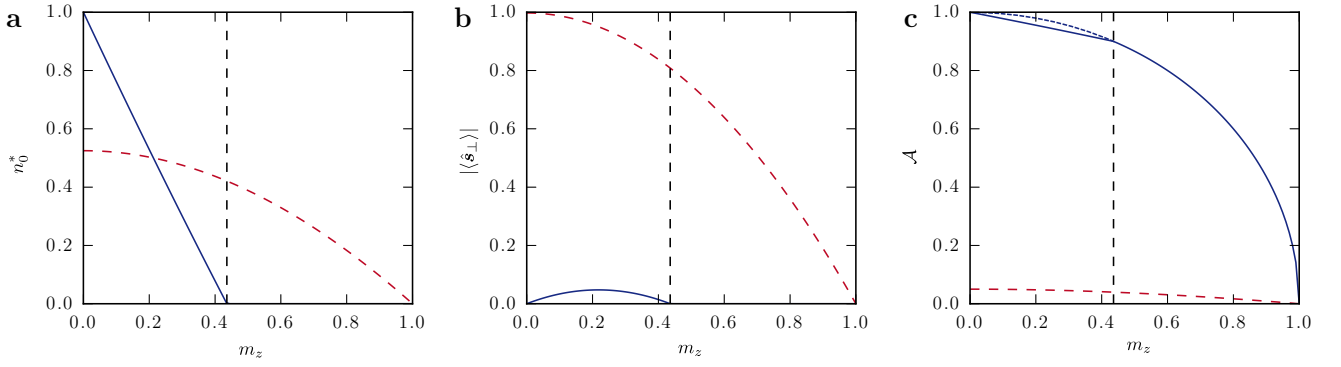

FIG. S11: **(a)** Equilibrium population  $n_0^*$ , **(b)** transverse spin length  $|\langle \hat{s}_\perp \rangle|$  and **(c)** alignment  $\mathcal{A}$  of an antiferromagnetic spin 1 condensate versus longitudinal magnetization  $m_z$ , for a fixed value of  $q/U_S = 0.2$  (solid lines). The dotted blue line in panel c indicates the maximum alignment  $\mathcal{A}_{\max}$ . The critical magnetization separating the broken axisymmetry from the antiferromagnetic phase is  $m_{z,c} = 0.6$ , marked by the black dashed line. For comparison, the dashed lines show the same quantities but for ferromagnetic interactions.

In the literature, it is common to call  $\mathbf{u}$  the director field. The tensor  $\overline{\overline{Q}}$ , or equivalently the director  $\mathbf{u}$ , plays the role of the order parameter for spin nematic states. The second limiting case is the one of an oriented or fully magnetized state, for which the average spin is maximal,  $|\langle \hat{\mathbf{s}} \rangle| = 1$ . This is achieved when  $|\mathbf{u}| = |\mathbf{v}| = 1/\sqrt{2}$ , and also corresponds to a non-zero spin quadrupole tensor

$$\overline{\overline{Q}} = \frac{1}{2} (\mathbb{1} - \underline{\mathbf{u}} \otimes \underline{\mathbf{u}}). \quad (\text{s28})$$

For a generic, partially magnetized state, one can quantify the proximity to one or the other limiting cases by the quantity  $\mathcal{A}$ , which characterizes the amount of alignment present in a given state. For purely aligned states  $\mathcal{A} = 1$  while for purely oriented states  $\mathcal{A} = 0$ . Since  $|\langle \hat{\mathbf{s}} \rangle|^2 = 4|\hat{\mathbf{u}}|^2|\hat{\mathbf{v}}|^2 = 4|\hat{\mathbf{u}}|^2(1 - |\hat{\mathbf{u}}|^2)$ , the alignment  $\mathcal{A}$  and spin length  $|\langle \hat{\mathbf{s}} \rangle|$  are related through the relation

$$|\langle \hat{\mathbf{s}} \rangle|^2 + \mathcal{A}^2 = 1. \quad (\text{s29})$$

### B. Application : ground state of spinor condensates

We use the same parametrization of the condensate spin wavefunction as in the main article, but written in the cartesian basis,

$$|\zeta\rangle = e^{i\theta_0} \begin{pmatrix} e^{i\Theta/2} [-A_- \cos(\alpha/2) - iA_+ \sin(\alpha/2)] \\ e^{i\Theta/2} [A_- \sin(\alpha/2) - iA_+ \cos(\alpha/2)] \\ B \end{pmatrix}, \quad (\text{s30})$$

where  $A_\pm = \frac{1}{2} (\sqrt{1 - n_0 + m_z} \pm \sqrt{1 - n_0 - m_z})$ ,  $B = \sqrt{n_0}$ . Note that  $A_-^2 + A_+^2 + B^2 = 1$ .

The average spin is then given by

$$\langle \hat{\mathbf{s}} \rangle = 2A_- \begin{pmatrix} -B \sin\left(\frac{\alpha}{2}\right) \\ -B \cos\left(\frac{\alpha}{2}\right) \\ A_+ \end{pmatrix}, \quad (\text{s31})$$

with a spin length  $|\langle \hat{\mathbf{s}} \rangle|^2 = 4A_-^2(1 - A_-^2)$ . The director  $\underline{\mathbf{u}}$  is given by

$$\underline{\mathbf{u}} = \frac{1}{\sqrt{1 - A_-^2}} \begin{pmatrix} A_+ \sin\left(\frac{\alpha}{2}\right) \\ A_+ \cos\left(\frac{\alpha}{2}\right) \\ B \end{pmatrix}. \quad (\text{s32})$$

Finally, the alignment is

$$\mathcal{A} = 1 - 2A_-^2 = n_0 + \sqrt{(1 - n_0)^2 - m_z^2}. \quad (\text{s33})$$

We show in Fig. S11 the equilibrium population  $n_0^*$  in the ground state of an antiferromagnetic condensate, together with the length  $|\langle \hat{s}_\perp \rangle|$  of the transverse spin and the alignment  $\mathcal{A}$ . Fig. S11c illustrates that  $\mathcal{A}$  stays close to the maximum value  $\mathcal{A}_{\text{max}} = \sqrt{1 - m_z^2}$  that the alignment can reach, given a magnetization  $m_z$ . This justifies using this quantity to determine the amount of alignment present in the state  $|\zeta\rangle$ , even when  $\langle \hat{s} \rangle \neq 0$ .

- 
- [1] D. Jacob, E. Mimoun, L. D. Sarlo, M. Weitz, J. Dalibard, and F. Gerbier, *New Journal of Physics* **13**, 065022 (2011).
  - [2] D. Jacob, L. Shao, V. Corre, T. Zibold, L. De Sarlo, E. Mimoun, J. Dalibard, and F. Gerbier, *Phys. Rev. A* **86**, 061601 (2012).
  - [3] W. Ketterle, D. S. Durfee, and D. M. Stamper-Kurn, in *Proceedings of the International School on Physics Enrico Fermi 1998, Bose-Einstein Condensation in Atomic Gases*, edited by M. Inguscio, S. Stringari, and C. E. Wieman (IOS Press, 1999), pp. 67–176, arXiv:cond-mat/9904034.
  - [4] H. Pu, C. K. Law, S. Raghavan, J. H. Eberly, and N. P. Bigelow, *Phys. Rev. A* **60**, 1463 (1999).
  - [5] M.-S. Chang, Q. Qin, W. Zhang, L. You, and M. S. Chapman, *Nature Physics* **1**, 111 (2005).
  - [6] J. Kronjäger, C. Becker, M. Brinkmann, R. Walser, P. Navez, K. Bongs, and K. Sengstock, *Physical Review A* **72**, 063619 (2005).
  - [7] W. Zhang, D. L. Zhou, M.-S. Chang, M. S. Chapman, and L. You, *Phys. Rev. A* **72**, 013602 (2005).
  - [8] A. T. Black, E. Gomez, L. D. Turner, S. Jung, and P. D. Lett, *Phys. Rev. Lett.* **99**, 070403 (2007).
  - [9] Y. Liu, S. Jung, S. E. Maxwell, L. D. Turner, E. Tiesinga, and P. D. Lett, *Phys. Rev. Lett.* **102**, 125301 (2009).
  - [10] V. Corre, T. Zibold, C. Frapolli, L. Shao, J. Dalibard, and F. Gerbier, *EPL* **110**, 26001 (2015).
  - [11] Y. Kawaguchi, N. T. Phuc, and P. B. Blakie, *Phys. Rev. A* **85**, 053611 (2012).
  - [12] S. Knoop, T. Schuster, R. Scelle, A. Trautmann, J. Appmeier, M. K. Oberthaler, E. Tiesinga, and E. Tiemann, *Phys. Rev. A* **83**, 042704 (2011).
  - [13] M. Naraschewski and D. M. Stamper-Kurn, *Phys. Rev. A* **58**, 2423 (1998).
  - [14] F. Dalfovo, S. Giorgini, L. P. Pitaevskii, and S. Stringari, *Rev. Mod. Phys.* **71**, 463 (1999).
  - [15] C. K. Law, H. Pu, and N. P. Bigelow, *Phys. Rev. Lett.* **81**, 5257 (1998).
  - [16] M. Koashi and M. Ueda, *Phys. Rev. Lett.* **84**, 1066 (2000).
  - [17] F. H. L. Essler, G. V. Shlyapnikov, and A. M. Tselik, *Journal of Statistical Mechanics* **02**, P02027 (2009).
  - [18] M. Snoek and F. Zhou, *Phys. Rev. B* **69**, 094410 (2004).
  - [19] M. Ueda, *Phys. Rev. A* **63**, 013601 (2000).
  - [20] C. J. Mullin, J. M. Keller, C. L. Hammer, and R. H. Good, *Annals of Physics* **37**, 55 (1966).
  - [21] B. A. Ivanov and A. K. Kolezhuk, *Phys. Rev. B* **68**, 052401 (2003).
  - [22] F. Zhou, M. Snoek, J. Wiemer, and I. Affleck, *Phys. Rev. B* **70**, 184434 (2004).
  - [23] A. Läuchli, F. Mila, and K. Penc, *Phys. Rev. Lett.* **97**, 087205 (2006).
  - [24] D. M. Stamper-Kurn and M. Ueda, *Rev. Mod. Phys.* **85**, 1191 (2013).
  - [25] This was verified in an independent calculation by solving the three-component, three-dimensional Gross-Pitaevskii (GP) equation
